# Supplementary material for: An embedded genus-one helicoid
Source: arXiv:math/0401080 source file (2004-06-04)
Supplement: Supplementary file 1 [file figs_inc_supp.tex]

\def\begfig {
\begin{figure}
\small
}
\def\endfig {
\normalsize
\end{figure}
}
